# Supplementary material for: PrivacEye: Privacy-Preserving Head-Mounted Eye Tracking Using Egocentric Scene Image and Eye Movement Features
Source: arXiv:1801.04457 source file (2019-05-24)
Supplement: Supplementary file 1 [file supplementary_material.pdf]

## Supplementary Material

# PrivacEye: Privacy-Preserving Head-Mounted Eye Tracking Using Egocentric Scene Image and Eye Movement Features

This supplementary document contains a detailed data annotation scheme description, an error case analysis, and the interview protocol analysing users' feedback towards PrivacEye.

## 1 DATA ANNOTATION SCHEME

Annotations were performed using Advene [Aubert et al. 2012]. Participants were asked to annotate continuous video segments showing the same situation, environment, or activity. They could also introduce new segments in case a privacy-relevant feature in the scene changed, e.g., when a participant switched to a sensitive app on the mobile phone. Participants were asked to annotate each of these segments according to the annotation scheme shown in Table 1, specifically scene content (Q1-7) and privacy sensitivity ratings (Q8). Privacy sensitivity was rated on a 7-point Likert scale (see Figure 1) ranging from 1 (fully inappropriate) to 7 (fully appropriate). As we expected our participants to have difficulties understanding the concept of "privacy sensitivity", we rephrased it for the annotation to "How appropriate is it that a camera is in the scene?".

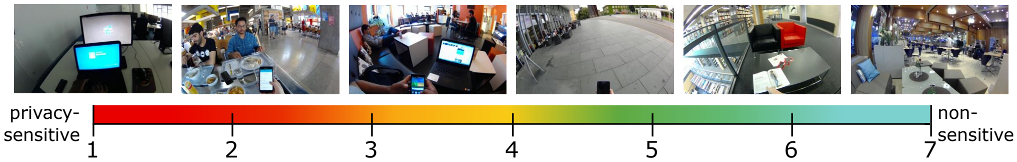


**Figure 1: Sample images showing daily situations ranging from "privacy-sensitive", such as password entry or social interactions, to "non-sensitive", such as walking down a road or sitting in a café.**

| # Question | Example Annotation |
|---|---|
| 1. What is the current environment you are in? | office, library, street, canteen |
| 2. Is this an indoor or outdoor environment? | indoor, outdoor |
| 3. What is your current activity in the video segment? | talking, texting, walking |
| 4. Are private objects present in the scene? | schedule, notes, wallet |
| 5. Are devices with potentially sensitive content present in the scene? | laptop, mobile phone |
| 6. Is a person present that you personally know? | yes, no |
| 7. Is the scene a public or a private place? | private, public, mixed |
| 8. How appropriate is it that a camera is in the scene? | Likert scale (1: fully inappropriate – 7: fully appropriate) |

**Table 1: Annotation scheme used by the participants to annotate their recordings.**

## 2 ERROR CASE ANALYSIS

For our system, it is not only important to detect the privacy-sensitive situations (TP), but equally important to detect non-sensitive situations (TN), which we are interested in recording while avoiding error cases.

Our results suggest that the combination *SVM/SVM* performs best for the person-specific case. In the following, we detail its performance on data recorded in different environments and during different activities. We detail on the occurrence of false positives, i.e., cases where the camera is de-activated in a non-sensitive situation, as well as false negatives, i.e., cases where the camera remains active although the scene is privacy-sensitive. Examples such as in Figure 2 show that, while false positives would be rather unproblematic in a realistic usage

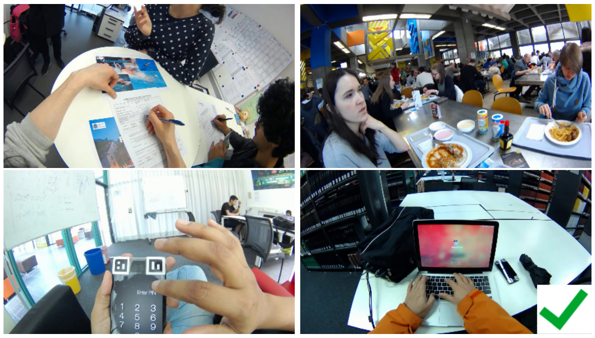

**(a) True positives**

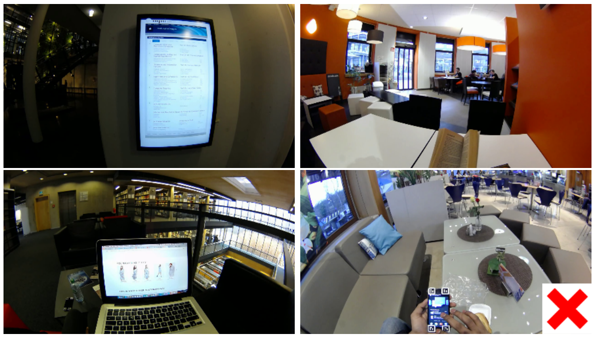

**(b) False positives**

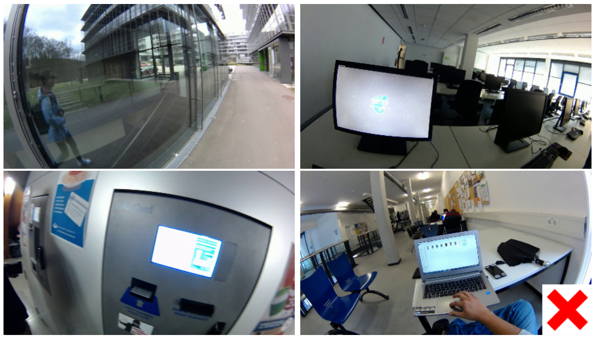

**(c) False negatives**

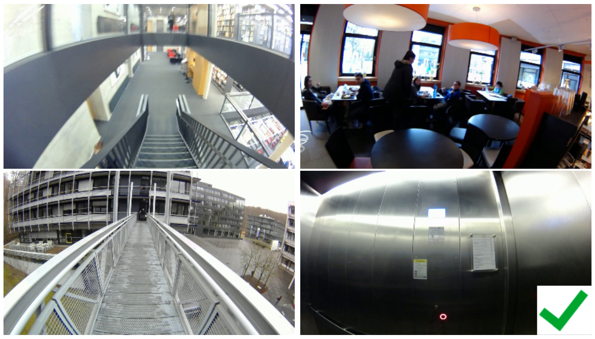

**(d) True negatives**

**Figure 2: Examples for (a) correct detection of "privacy-sensitive" situations, (b) incorrect detection of "non-sensitive" situations, (c) incorrect detection of "privacy-sensitive" situations, and (d) correct detection of "non-sensitive" situations.**

scenario, false negatives are critical and might lead to misclosures. Thus, our argumentation focuses on eliminating false negatives. While PrivacEye correctly identifies signing a document, social interactions, and screen interactions as privacy-sensitive, false positives contain reading a book or standing in front of a public display. In these cases PrivacEye would act too restrictively in cases where de-activating the camera would lead to a loss of functionality (e.g. tracking). False negative cases include, e.g., reflections (when standing in front of a window), self-luminous screens, or cases that are under-represented in our data set (e.g. entering a pin at the ATM).

Figure 3 provides a detailed overview of true positives and false negatives with respect to the labelled environments (3, left) and activities (3, right). For each label two stacked bars are shown: PrivacEye's prediction (top row) and the ground truth annotation (GT, bottom row). The prediction's result defines the "cut-off" between closed shutter (left, privacy-sensitive) and open shutter (right, non-sensitive), which is displayed as vertical bar. Segments that were predicted to be privacy-sensitive, include both true positives (TP, red) and false positives (FP, orange) are shown left of the "cut-off". Similarly, those segments that were predicted to be non-sensitive, including true negatives (TN, yellow-green) and false negatives (FN, red), are displayed right of the "cut-off". While false positives (FP) (i.e., non-sensitive situations classified as sensitive) are not problematic, as they to not create the risk of misclosures, false negatives (FN) are critical. Thus, we focus our discussion on the false negatives (red, top, right). A comparison of true positives (TP) and false negatives (FN) shows that PrivacEye performs well within most environments, e.g., offices or corridors. In these environments true positives outweigh false negatives. However, in the computer room environment, where a lot of screens with potentially problematic content (which the wearer might not even be aware of at recording time) are present, performance drops. Misclassifications between personal displays, e.g., laptops and public displays (e.g. room occupancy plans) are a likely reason for the larger amount of false negatives (FN). Future work might aim to combine PrivacEye with an image-based classifier trained for screen contents (c.f., [Korayem et al. 2016]), which, however, would come at the cost of excluding also non-sensitive screens from the footage. Future work might specifically target these situations to increase accuracy. For the activities outlined in Figure 3 (left), PrivacEye works best while eating/drinking and in media interactions. Also, the results are promising for detecting social interactions. The performance for password entry, however, is still limited. Although the results show that it is possible to detect password entry, the amount of true negatives (TN) is comparatively high. This is likely caused by the under-representation of this activity, which typically lasts only a few seconds in our data set. Future work might be able to eliminate this by specifically training for password and PIN entry, possibly enabling the classifier to better distinguish between PIN entry and, e.g., reading.

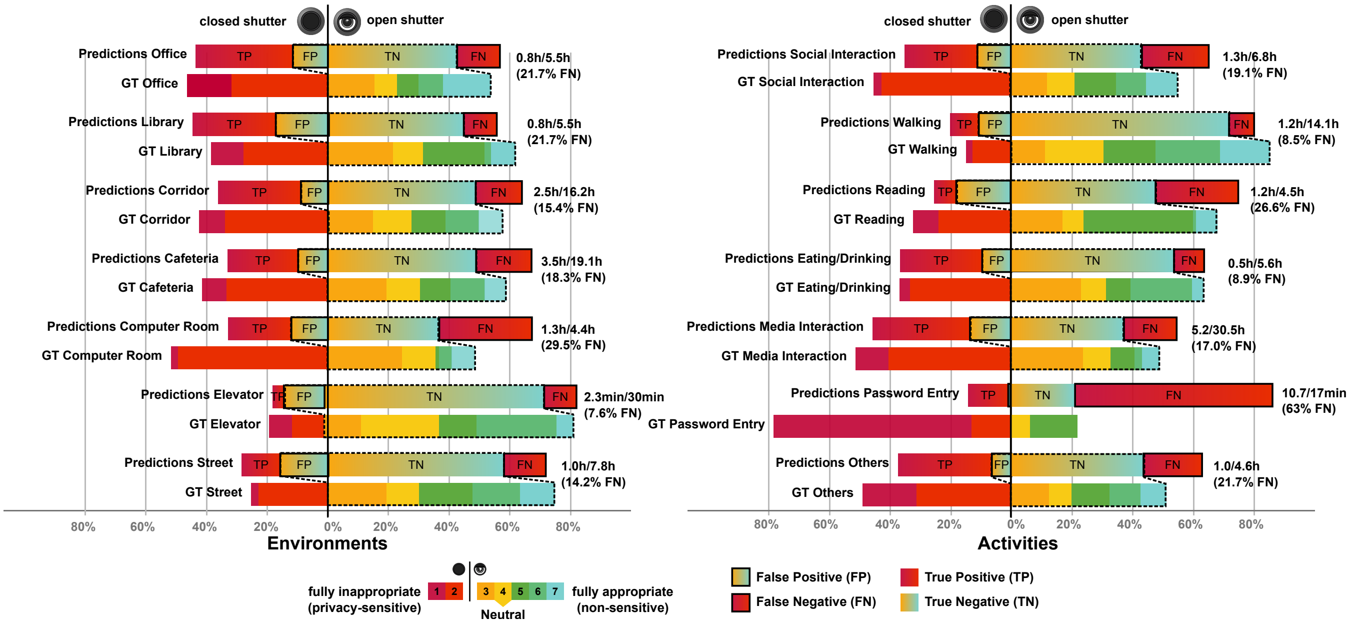


**Figure 3: Error case analysis for different environments (left) and activities (right) showing the "cut-off" between closed shutter (left, *privacy-sensitive*) and open shutter (right, *non-sensitive*) with PrivacEye prediction and the corresponding ground truth (GT). False positives (FP) are *non-sensitive* but protected (closed shutter), false negatives (FN) are *privacy-sensitive* but unprotected (open shutter).**

## 3 INTERVIEW PROTOCOL

During the interviews, participants were encouraged to interact with state-of-the-art head-mounted displays (Vuzix M300 and Sony SmartEyeglass) and our prototype. Participants were presented with the fully functional PrivacEye prototype, which was used to illustrate three scenarios: 1) interpersonal conversations, 2) sensitive objects (a credit card and a passport), and 3) sensitive contents on a device screen. Due to the time required to gather person-specific training data for each interviewee as well as runtime restrictions, the scenarios were presented using the Wizard-of-Oz method. This is also advantageous, as the laboratory-style study environment – with white walls, an interviewer and no distractors present – might have induced different eye movement patterns than a natural environment. Also, potential errors of the system, caused by its prototypical implementation, might have caused participant bias toward the concept. To prevent these issues, the shutter was controlled remotely by an experimental assistant. This way, the interviewees commented on the concept and vision of PrivacEye and not on the actual proof-of-concept implementation, which – complementing the afore-described evaluation – provides a more comprehensive and universal set of results altogether. The semi-structured interview was based on the following questions:

Q1 *Would you be willing to wear something that would block someone from being able to record you?*
Q2 *If technically feasible, would you expect the devices themselves, instead of their user, to protect your privacy automatically?*
Q3 *Would you feel different about being around someone who is wearing those kinds of intelligent glasses than about those commercially available today? Why?*
Q4 *If you were using AR glasses, would you be concerned about accidentally recording any sensitive information belonging to you?*
Q5 *How would you feel about (such) a system automatically taking care that you do not capture any sensitive information?*
Q6 *How do you think the eye tracking works? What can the system infer from your eye data?*
Q7 *How would you feel about having your eye movements tracked by augmented reality glasses?*

The questions were designed following a "funnel principle", with increasing specificity towards the end of the interview. We started with four more general questions (not listed above), such as "Do you think recording with those glasses is similar or different to recording with a cell phone? Why?", based on [Denning et al. 2014]. This provided the participant with some time to familiarize herself with the topic before being presented with the proof-of-concept prototype (use case "bystander privacy") after Q1 and the use cases "sensitive objects" (e.g., credit card, passport) and "sensitive data" (e.g. login data) after Q4. Eye tracking functionality was demonstrated after Q5. While acquiescence and other forms of interviewer effects cannot be ruled out completely, this step-by-step presentation of the prototype and its scenarios ensured that the participants voiced their own ideas first, before being directed towards discussing the actual concept of the PrivacEye prototype. Each participant was asked for his/her perspectives on the PrivacEye's concept (Q2-Q5) and eye tracking (Q6 and Q7). The interviews were audio recorded and transcribed for later analysis. Subsequently, qualitative analysis was performed following inductive category development [Mayring 2014]. Key motives and reoccurring themes were extracted and are presented in this section.

## REFERENCES


Olivier Aubert, Yannick Prié, and Daniel Schmitt. 2012. Advene As a Tailorable Hypervideo Authoring Tool: A Case Study. In *Proceedings of the 2012 ACM Symposium on Document Engineering (DocEng '12)*. ACM, New York, NY, USA, 79–82. https://doi.org/10.1145/2361354.2361370

Tamara Denning, Zakariya Dehlawi, and Tadayoshi Kohno. 2014. In situ with Bystanders of Augmented Reality Glasses: Perspectives on Recording and Privacy-mediating Technologies. In *Proceedings of the Conference on Human Factors in Computing Systems (CHI)*. ACM, 2377–2386. https://doi.org/10.1145/2556288.2557352

Mohammed Korayem, Robert Templeman, Dennis Chen, David Crandall, and Apu Kapadia. 2016. Enhancing lifelogging privacy by detecting screens. In *Proceedings of the 2016 CHI Conference on Human Factors in Computing Systems*. ACM, 4309–4314. https://doi.org/10.1145/2702123.2702183

Philipp Mayring. 2014. *Qualitative content analysis: theoretical foundation, basic procedures and software solution.* 143 pages. https://doi.org/10.1007/978-94-017-9181-6_13
